# Supplementary material for: Recovering 3D Hand Mesh Sequence from a Single Blurry Image: A New Dataset and Temporal Unfolding
Source: arXiv:2303.15417 source file (2023-03-27)
Supplement: Supplementary file 1 [file YT3D_comparison_last.tex]

% \begin{figure*}[t]
%     \centering
%     \newcommand{\spacing}{3.0cm}
%     \captionsetup[subfigure]{labelfont=scriptsize, textfont=scriptsize}
%     %     \hspace*{\fill}
%     %     \subfloat{\includegraphics[width=\spacing]{latex/supple/figures/YT3D/10200_B_img.png}}
%     %     \hfill
%     %     \subfloat{\includegraphics[width=\spacing]{latex/supple/figures/YT3D/10200_D_img.png}}
%     %     \hfill
%     %     \subfloat{\includegraphics[width=\spacing]{latex/supple/figures/YT3D/10200_S_mesh.png}}
%     %     \hfill
%     %     \subfloat{\includegraphics[width=\spacing]{latex/supple/figures/YT3D/10200_D_mesh.png}}
%     %     \hfill
%     %     \subfloat{\includegraphics[width=\spacing]{latex/supple/figures/YT3D/10200_B_mesh.png}}
%     %     \hspace*{\fill}
%     % \\
%     %     \hspace*{\fill}
%     %     \subfloat{\includegraphics[width=\spacing]{latex/supple/figures/YT3D/11166_B_img.png}}
%     %     \hfill
%     %     \subfloat{\includegraphics[width=\spacing]{latex/supple/figures/YT3D/11166_D_img.png}}
%     %     \hfill
%     %     \subfloat{\includegraphics[width=\spacing]{latex/supple/figures/YT3D/11166_S_mesh.png}}
%     %     \hfill
%     %     \subfloat{\includegraphics[width=\spacing]{latex/supple/figures/YT3D/11166_D_mesh.png}}
%     %     \hfill
%     %     \subfloat{\includegraphics[width=\spacing]{latex/supple/figures/YT3D/11166_B_mesh.png}}
%     %     \hspace*{\fill}
%     % \\
%     %     \hspace*{\fill}
%     %     \subfloat{\includegraphics[width=\spacing]{latex/supple/figures/YT3D/11266_B_img.png}}
%     %     \hfill
%     %     \subfloat{\includegraphics[width=\spacing]{latex/supple/figures/YT3D/11266_D_img.png}}
%     %     \hfill
%     %     \subfloat{\includegraphics[width=\spacing]{latex/supple/figures/YT3D/11266_S_mesh.png}}
%     %     \hfill
%     %     \subfloat{\includegraphics[width=\spacing]{latex/supple/figures/YT3D/11266_D_mesh.png}}
%     %     \hfill
%     %     \subfloat{\includegraphics[width=\spacing]{latex/supple/figures/YT3D/11266_B_mesh.png}}
%     %     \hspace*{\fill}
%     % \\
%         \subfloat{\includegraphics[width=\spacing]{latex/supple/figures/YT3D/29022_B_img.png}}
%         \hfill
%         \subfloat{\includegraphics[width=\spacing]{latex/supple/figures/YT3D/29022_D_img.png}}
%         \hfill
%         \subfloat{\includegraphics[width=\spacing]{latex/supple/figures/YT3D/29022_S_mesh.png}}
%         \hfill
%         \subfloat{\includegraphics[width=\spacing]{latex/supple/figures/YT3D/29022_D_mesh.png}}
%         \hfill
%         \subfloat{\includegraphics[width=\spacing]{latex/supple/figures/YT3D/29022_B_mesh.png}}
%     \\
%         \subfloat{\includegraphics[width=\spacing]{latex/supple/figures/YT3D/30828_B_img.png}}
%         \hfill
%         \subfloat{\includegraphics[width=\spacing]{latex/supple/figures/YT3D/30828_D_img.png}}
%         \hfill
%         \subfloat{\includegraphics[width=\spacing]{latex/supple/figures/YT3D/30828_S_mesh.png}}
%         \hfill
%         \subfloat{\includegraphics[width=\spacing]{latex/supple/figures/YT3D/30828_D_mesh.png}}
%         \hfill
%         \subfloat{\includegraphics[width=\spacing]{latex/supple/figures/YT3D/30828_B_mesh.png}}
%     \\
%         \subfloat{\includegraphics[width=\spacing]{latex/supple/figures/YT3D/29824_B_img.png}}
%         \hfill
%         \subfloat{\includegraphics[width=\spacing]{latex/supple/figures/YT3D/29824_D_img.png}}
%         \hfill
%         \subfloat{\includegraphics[width=\spacing]{latex/supple/figures/YT3D/29824_S_mesh.png}}
%         \hfill
%         \subfloat{\includegraphics[width=\spacing]{latex/supple/figures/YT3D/29824_D_mesh.png}}
%         \hfill
%         \subfloat{\includegraphics[width=\spacing]{latex/supple/figures/YT3D/29824_B_mesh.png}}
%     \addtocounter{subfigure}{-15}
%     \\
%         \subfloat[Blurry image]{\includegraphics[width=\spacing]{latex/supple/figures/YT3D/11557_B_img.png}}
%         \hfill
%         \subfloat[Deblurred image]{\includegraphics[width=\spacing]{latex/supple/figures/YT3D/11557_D_img.png}}
%         \hfill
%         \subfloat[IH2.6M + YT3D]{\includegraphics[width=\spacing]{latex/supple/figures/YT3D/11557_S_mesh.png}}
%         \hfill
%         \subfloat[BH+\textbf{D} + YT3D]{\includegraphics[width=\spacing]{latex/supple/figures/YT3D/11557_D_mesh.png}}
%         \hfill
%         \subfloat[BH + YT3D]{\includegraphics[width=\spacing]{latex/supple/figures/YT3D/11557_B_mesh.png}}
%     % \\
% \vspace{-2mm}
%     \caption{\textbf{Effectiveness of the presented BlurHand.}
%     The captions below figures describe training sets used to train 3D hand mesh estimation networks.
%     A setting with \textbf{D} represents that the network is trained on deblurred BH and tested on (b).
%     }
%     \vspace{-0.4cm}
%     \label{fig:supple_comparison_yt3d}
% \end{figure*}
