# Supplementary material for: Recovering 3D Hand Mesh Sequence from a Single Blurry Image: A New Dataset and Temporal Unfolding
Source: arXiv:2303.15417 source file (2023-03-27)
Supplement: Supplementary file 2 [file 1_video_format.tex]

\section{Visualization in video format}
\label{sec_supp:video_results}
% 
% We present the video clips showing the recovered 3D meshes of our BlurHandNet with the blurry input in the supplementary videos~(\textbf{\fontfamily{pcr}\selectfont BlurHandNet.mp4}).
In the supplementary videos~(\textbf{\fontfamily{pcr}\selectfont BlurHandNet.mp4}), we visualize the recovered 3D hand mesh sequence as video clips. 
In the video, we note that the left part is the input blurry hand image, and the right part is the results from our BlurHandNet.
We further note that we adopt linear interpolation to smooth the motion, and motion order is determined in the order of $\mathbf{V}_{\text{E1}}$, $\mathbf{V}_{\text{M}}$, and $\mathbf{V}_{\text{E2}}$.

The video shows that our BlurHandNet outputs robust 3D hand meshes from challenging blurry hand.
Moreover, our BlurHandNet successfully estimates the motion in the blurry hand by performing temporal unfolding through the proposed Unfolder.
Compared to the previous methods, which output the mesh in the static scene, our BlurHandNet gives more accurate and comprehensive results from blurry inputs, including motion information.
